# Supplementary material for: Estimation of Long-Range Dependent Models with Missing Data: to Impute or not to Impute?
Source: arXiv:2303.04754 source file (2026-05-07)
Supplement: Supplementary file 1 [file Supplementary_Material.pdf]

# Estimation of Long-Range Dependent Models with Missing Data: to Input or not to Input?

## Supplementary Material

Guilherme Pumi<sup>a,\*</sup>, Gladys Choque Ulloa<sup>a</sup> and Taiane Schaedler Prass<sup>a</sup>

This supplementary material is intended to present some complementary results to the ones presented in the parent paper. Henceforth, We shall apply the same notation, nomenclature, and abbreviations as in the main paper without further mention or reference. To the interested reader we refer the main paper for details.

The results presented here cover two main scenarios. The first one is the case of simulated ARFIMA(0,  $d$ , 0), for which we present the cases the case  $d \in \{0.1, 0.4\}$  in the main paper and  $d \in \{0.2, 0.3\}$  here. The results presented here are very similar to the ones presented in the paper. The discussion presented in the paper for the case  $d = 0.1$  apply viz-a-viz to the case  $d = 0.2$  here. The results for  $d = 0.3$  presented here are very similar to those for  $d = 0.4$  discussed in the main paper.

The second main scenario is the case of simulated ARFIMA(1,  $d$ , 1), which is presented here. Since the estimators applied in the paper are semiparametric, the AR and MA contribution to the estimation of  $d$  should, in principle, be negligible. It is indeed the case and the results of every scenario simulated for the ARFIMA(1,  $d$ , 1) are similar to the respective ARFIMA(0,  $d$ , 0) counterpart. Hence, the discussion presented in the paper for the ARFIMA(0,  $d$ , 0) apply viz-a-viz to the (1,  $d$ , 1) case presented here.

---

\*Corresponding author. This Version: March 8, 2023

<sup>a</sup>Programa de Pós-Graduação em Estatística - Universidade Federal do Rio Grande do Sul.

E-mails: guilherme.pumi@ufrgs.br (G. Pumi), gladyschoqueulloa7@gmail.com (G. U. Choque) and tianeprass@ufrgs.br (T. S. Prass)

# 1 ARFIMA(0, $d$ , 0) scenario

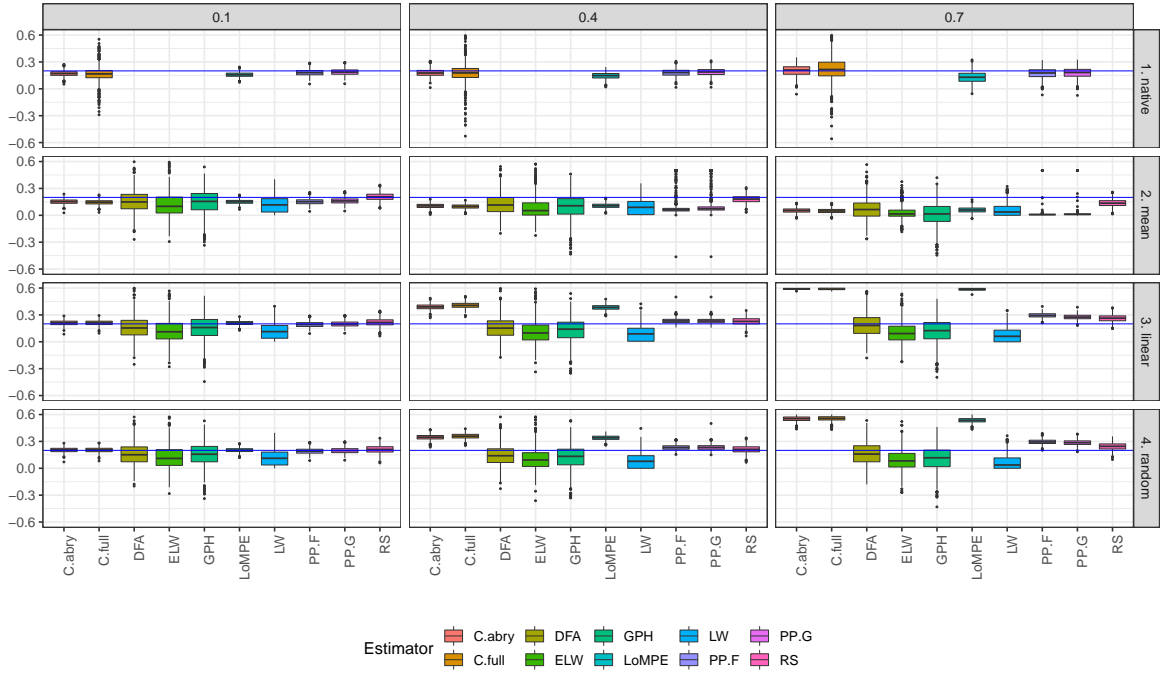

Figure 1: Box plot of the adjusted model ARFIMA (0,  $d$ , 0) for  $d = 0.2$ .

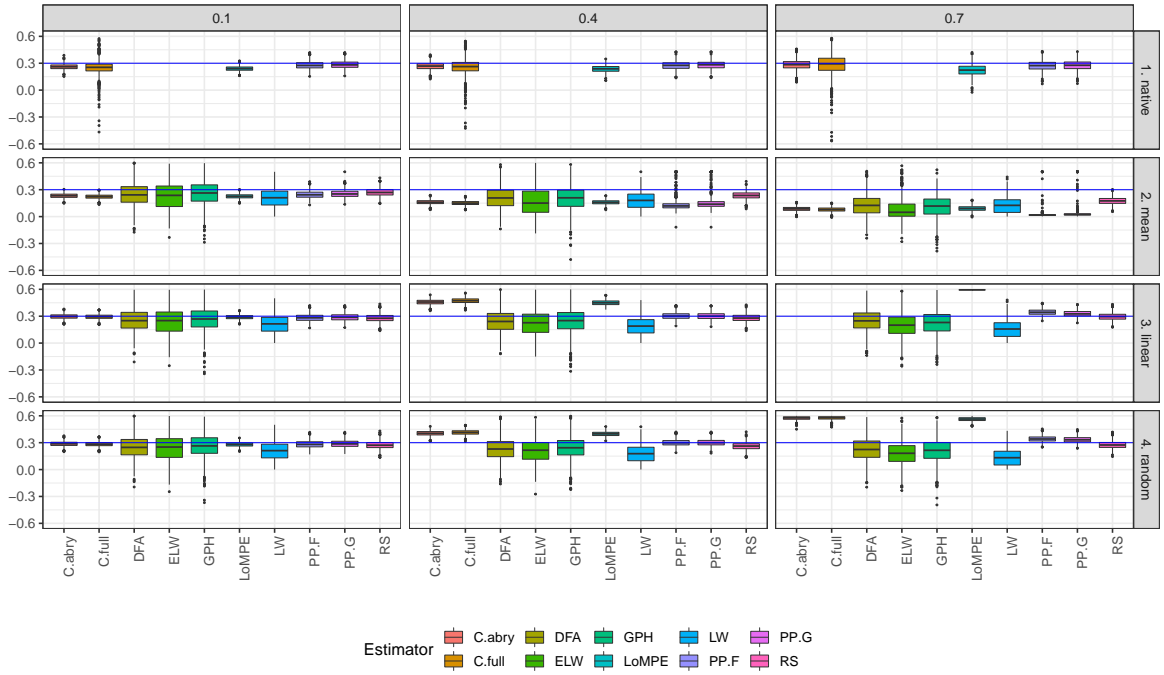

Figure 2: Box plot of the adjusted model ARFIMA (0,  $d$ , 0) for  $d = 0.3$ .

Table 1: Simulation results for the ARFIMA (0, 0.2, 0) scenario.

| $d = 0.2$ |           |              |              |              |              |              |              |              |              |
|-----------|-----------|--------------|--------------|--------------|--------------|--------------|--------------|--------------|--------------|
| Type      | Estimator | Missing      |              |              |              |              |              |              |              |
|           |           | 0            | 0.1          | 0.2          | 0.3          | 0.4          | 0.5          | 0.6          | 0.7          |
| Native    | Full      | 0.160        | 0.164        | 0.164        | 0.170        | 0.181        | <b>0.190</b> | <b>0.197</b> | 0.225        |
|           | Abry      | 0.167        | 0.171        | 0.171        | 0.175        | 0.178        | 0.182        | 0.185        | <b>0.203</b> |
|           | PP.G      | <b>0.188</b> | <b>0.188</b> | <b>0.187</b> | <b>0.186</b> | <b>0.187</b> | 0.183        | 0.181        | 0.177        |
|           | PP.F      | 0.181        | 0.181        | 0.180        | 0.179        | 0.180        | 0.177        | 0.175        | 0.173        |
|           | LoMPE     | 0.164        | 0.157        | 0.151        | 0.144        | 0.145        | 0.136        | 0.127        | 0.127        |
| Mean      | Full      | 0.160        | 0.146        | 0.130        | 0.114        | 0.098        | 0.083        | 0.064        | 0.048        |
|           | Abry      | 0.167        | 0.152        | 0.136        | 0.121        | 0.105        | 0.089        | 0.070        | 0.053        |
|           | PP.G      | <b>0.188</b> | 0.161        | 0.131        | 0.102        | 0.114        | 0.092        | 0.030        | 0.015        |
|           | PP.F      | 0.181        | 0.152        | 0.120        | 0.090        | 0.095        | 0.066        | 0.023        | 0.011        |
|           | LoMPE     | 0.164        | 0.151        | 0.136        | 0.121        | 0.106        | 0.091        | 0.074        | 0.060        |
|           | DFA       | 0.164        | 0.156        | 0.143        | 0.132        | 0.121        | 0.104        | 0.087        | 0.066        |
|           | GPH       | 0.158        | 0.148        | 0.128        | 0.111        | 0.094        | 0.069        | 0.042        | 0.011        |
|           | LW        | 0.123        | 0.118        | 0.108        | 0.102        | 0.096        | 0.082        | 0.070        | 0.058        |
|           | ELW       | 0.130        | 0.120        | 0.106        | 0.094        | 0.085        | 0.072        | 0.071        | 0.081        |
|           | R/S       | 0.216        | <b>0.207</b> | <b>0.200</b> | <b>0.189</b> | <b>0.181</b> | <b>0.168</b> | <b>0.154</b> | <b>0.136</b> |
| Linear    | Full      | 0.160        | 0.212        | 0.268        | 0.333        | 0.407        | 0.494        | 0.587        | 0.707        |
|           | Abry      | 0.167        | 0.212        | 0.262        | 0.321        | 0.389        | 0.471        | 0.563        | 0.685        |
|           | PP.G      | <b>0.188</b> | <b>0.200</b> | 0.210        | 0.221        | 0.233        | 0.243        | 0.258        | 0.277        |
|           | PP.F      | 0.181        | 0.194        | <b>0.206</b> | <b>0.219</b> | 0.234        | 0.249        | 0.269        | 0.295        |
|           | LoMPE     | 0.164        | 0.210        | 0.260        | 0.318        | 0.383        | 0.461        | 0.551        | 0.669        |
|           | DFA       | 0.164        | 0.160        | 0.156        | 0.155        | 0.156        | 0.152        | <b>0.162</b> | <b>0.184</b> |
|           | GPH       | 0.158        | 0.155        | 0.143        | 0.135        | 0.132        | 0.118        | 0.124        | 0.116        |
|           | LW        | 0.123        | 0.118        | 0.109        | 0.104        | 0.096        | 0.084        | 0.080        | 0.077        |
|           | ELW       | 0.130        | 0.127        | 0.120        | 0.112        | 0.109        | 0.096        | 0.096        | 0.101        |
|           | R/S       | 0.216        | 0.217        | 0.219        | 0.222        | <b>0.228</b> | <b>0.234</b> | 0.246        | 0.263        |
| Random    | Full      | 0.160        | 0.204        | 0.250        | 0.302        | 0.358        | 0.420        | 0.485        | 0.563        |
|           | Abry      | 0.167        | 0.205        | 0.245        | 0.293        | 0.346        | 0.407        | 0.474        | 0.557        |
|           | PP.G      | <b>0.188</b> | <b>0.198</b> | 0.209        | 0.220        | 0.234        | 0.247        | 0.265        | 0.286        |
|           | PP.F      | 0.181        | 0.192        | <b>0.204</b> | 0.217        | 0.232        | 0.249        | 0.270        | 0.295        |
|           | LoMPE     | 0.164        | 0.203        | 0.243        | 0.290        | 0.340        | 0.397        | 0.460        | 0.536        |
|           | DFA       | 0.164        | 0.156        | 0.148        | 0.143        | 0.143        | 0.139        | 0.144        | <b>0.163</b> |
|           | GPH       | 0.158        | 0.153        | 0.136        | 0.130        | 0.123        | 0.110        | 0.111        | 0.107        |
|           | LW        | 0.123        | 0.116        | 0.103        | 0.098        | 0.087        | 0.074        | 0.070        | 0.065        |
|           | ELW       | 0.130        | 0.124        | 0.115        | 0.109        | 0.103        | 0.091        | 0.090        | 0.090        |
|           | R/S       | 0.216        | 0.211        | 0.210        | <b>0.208</b> | <b>0.212</b> | <b>0.216</b> | <b>0.226</b> | 0.244        |

Table 2: Simulated results for the ARFIMA(0, 0.3, 0) scenario

| $d = 0.3$ |           |              |              |              |              |              |              |              |              |
|-----------|-----------|--------------|--------------|--------------|--------------|--------------|--------------|--------------|--------------|
| Type      | Estimator | Missing      |              |              |              |              |              |              |              |
|           |           | 0            | 0.1          | 0.2          | 0.3          | 0.4          | 0.5          | 0.6          | 0.7          |
| Native    | Full      | 0.247        | 0.255        | 0.264        | 0.277        | 0.241        | 0.272        | 0.269        | <b>0.296</b> |
|           | Abry      | 0.256        | 0.261        | 0.263        | 0.264        | 0.266        | 0.270        | 0.273        | 0.283        |
|           | PP.G      | <b>0.284</b> | <b>0.283</b> | <b>0.284</b> | <b>0.282</b> | <b>0.282</b> | <b>0.280</b> | <b>0.278</b> | 0.275        |
|           | PP.F      | 0.278        | 0.277        | 0.278        | 0.277        | 0.277        | 0.275        | 0.274        | 0.271        |
|           | LoMPE     | 0.248        | 0.240        | 0.237        | 0.227        | 0.237        | 0.226        | 0.215        | 0.223        |
| Mean      | Full      | 0.247        | 0.223        | 0.200        | 0.175        | 0.151        | 0.128        | 0.103        | 0.079        |
|           | Abry      | 0.256        | 0.233        | 0.210        | 0.185        | 0.161        | 0.138        | 0.112        | 0.086        |
|           | PP.G      | <b>0.284</b> | 0.255        | 0.220        | 0.182        | 0.167        | 0.123        | 0.058        | 0.033        |
|           | PP.F      | 0.278        | 0.245        | 0.207        | 0.166        | 0.144        | 0.102        | 0.046        | 0.023        |
|           | LoMPE     | 0.248        | 0.226        | 0.204        | 0.181        | 0.159        | 0.138        | 0.115        | 0.090        |
|           | DFA       | 0.263        | 0.251        | 0.243        | 0.225        | 0.211        | 0.190        | 0.161        | 0.129        |
|           | GPH       | 0.273        | 0.257        | 0.247        | 0.227        | 0.203        | 0.179        | 0.149        | 0.108        |
|           | LW        | 0.216        | 0.208        | 0.203        | 0.190        | 0.179        | 0.167        | 0.147        | 0.125        |
|           | ELW       | 0.252        | 0.235        | 0.219        | 0.199        | 0.176        | 0.159        | 0.138        | 0.121        |
|           | R/S       | 0.280        | <b>0.271</b> | <b>0.261</b> | <b>0.250</b> | <b>0.236</b> | <b>0.220</b> | <b>0.200</b> | <b>0.175</b> |
| Linear    | Full      | 0.247        | 0.293        | 0.346        | 0.406        | 0.473        | 0.551        | 0.643        | 0.755        |
|           | Abry      | 0.256        | <b>0.296</b> | 0.342        | 0.395        | 0.457        | 0.531        | 0.621        | 0.733        |
|           | PP.G      | <b>0.284</b> | 0.288        | <b>0.292</b> | <b>0.297</b> | <b>0.302</b> | <b>0.308</b> | 0.316        | 0.328        |
|           | PP.F      | 0.278        | 0.283        | 0.289        | 0.295        | 0.303        | 0.312        | 0.326        | 0.345        |
|           | LoMPE     | 0.248        | 0.289        | 0.337        | 0.388        | 0.450        | 0.522        | 0.607        | 0.712        |
|           | DFA       | 0.263        | 0.258        | 0.256        | 0.250        | 0.246        | 0.241        | 0.242        | 0.254        |
|           | GPH       | 0.273        | 0.266        | 0.262        | 0.256        | 0.248        | 0.238        | 0.234        | 0.225        |
|           | LW        | 0.216        | 0.210        | 0.206        | 0.197        | 0.189        | 0.178        | 0.167        | 0.157        |
|           | ELW       | 0.252        | 0.246        | 0.242        | 0.236        | 0.224        | 0.215        | 0.207        | 0.198        |
|           | R/S       | 0.280        | 0.279        | 0.279        | 0.279        | 0.280        | 0.281        | <b>0.286</b> | <b>0.295</b> |
| Random    | Full      | 0.247        | 0.284        | 0.324        | 0.367        | 0.415        | 0.468        | 0.527        | 0.593        |
|           | Abry      | 0.256        | <b>0.287</b> | 0.322        | 0.360        | 0.405        | 0.458        | 0.518        | 0.589        |
|           | PP.G      | <b>0.284</b> | <b>0.287</b> | <b>0.291</b> | <b>0.296</b> | <b>0.301</b> | <b>0.309</b> | <b>0.319</b> | 0.333        |
|           | PP.F      | 0.278        | 0.282        | 0.287        | 0.293        | <b>0.301</b> | 0.310        | 0.323        | 0.342        |
|           | LoMPE     | 0.248        | 0.280        | 0.317        | 0.354        | 0.398        | 0.448        | 0.503        | 0.567        |
|           | DFA       | 0.263        | 0.254        | 0.249        | 0.239        | 0.231        | 0.223        | 0.221        | 0.227        |
|           | GPH       | 0.273        | 0.263        | 0.256        | 0.250        | 0.238        | 0.223        | 0.217        | 0.209        |
|           | LW        | 0.216        | 0.207        | 0.200        | 0.188        | 0.176        | 0.164        | 0.151        | 0.136        |
|           | ELW       | 0.252        | 0.245        | 0.236        | 0.228        | 0.212        | 0.203        | 0.190        | 0.180        |
|           | R/S       | 0.280        | 0.274        | 0.269        | 0.265        | 0.262        | 0.260        | 0.263        | <b>0.276</b> |

## 2 ARFIMA(1, $d$ , 1) scenario

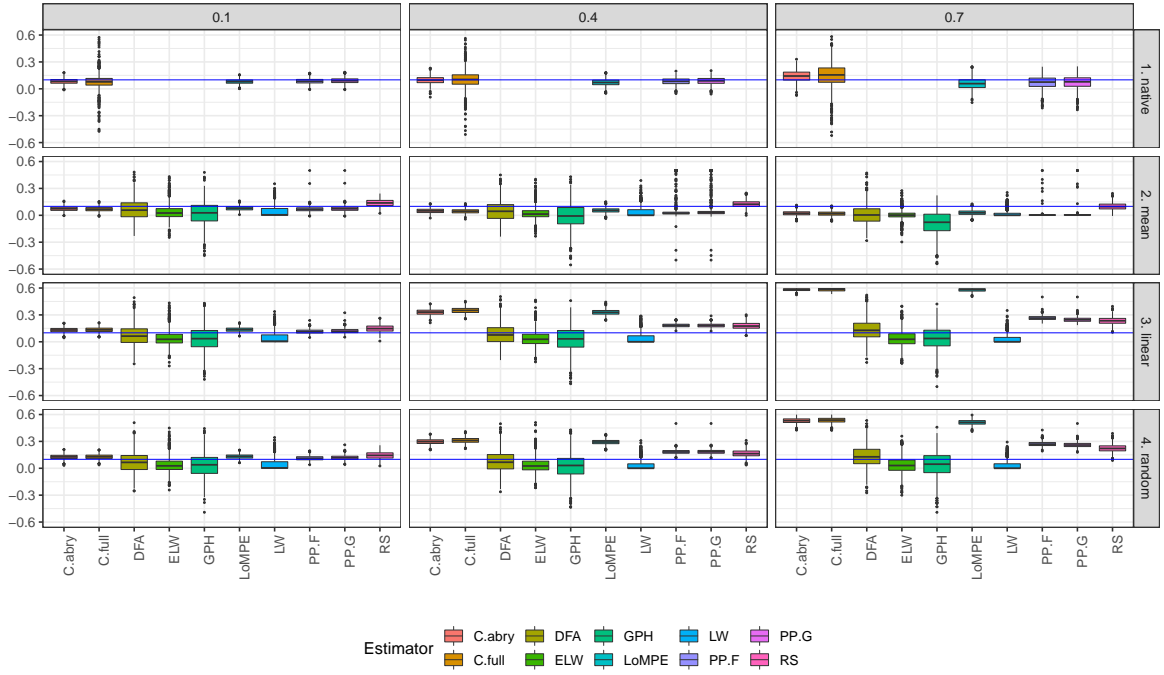

Figure 3: Box plot of the adjusted model ARFIMA (1,  $d$ , 1) for  $d = 0.1$ .

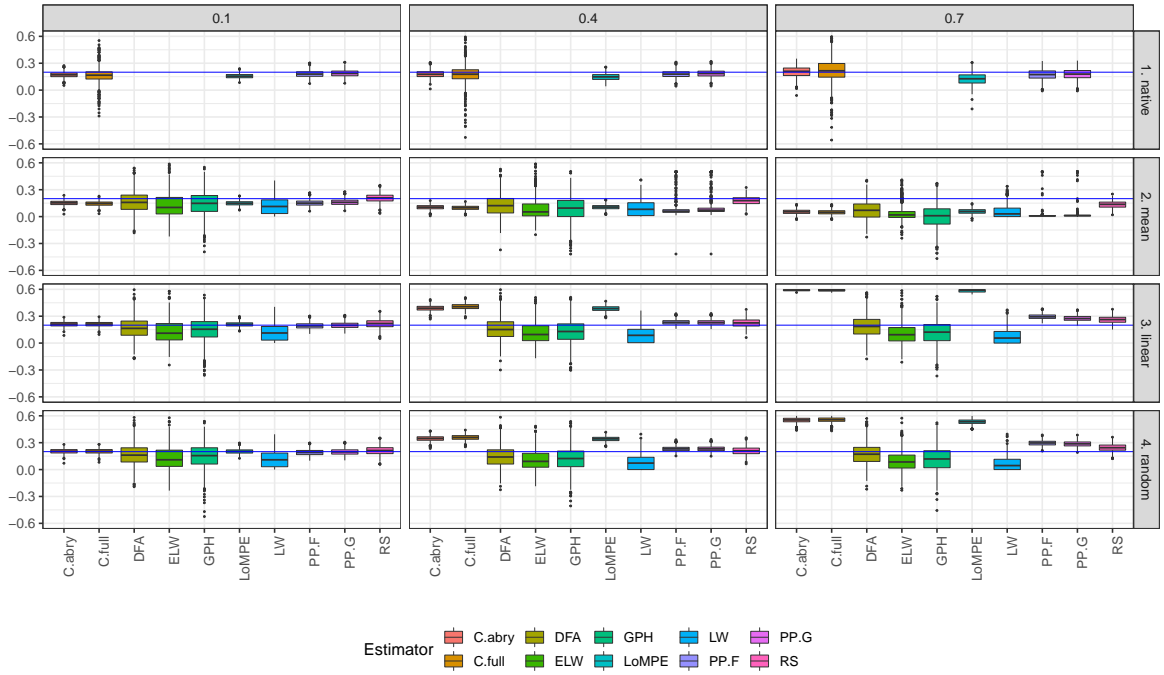

Figure 4: Box plot of the adjusted model ARFIMA (1,  $d$ , 1) for  $d = 0.2$ .

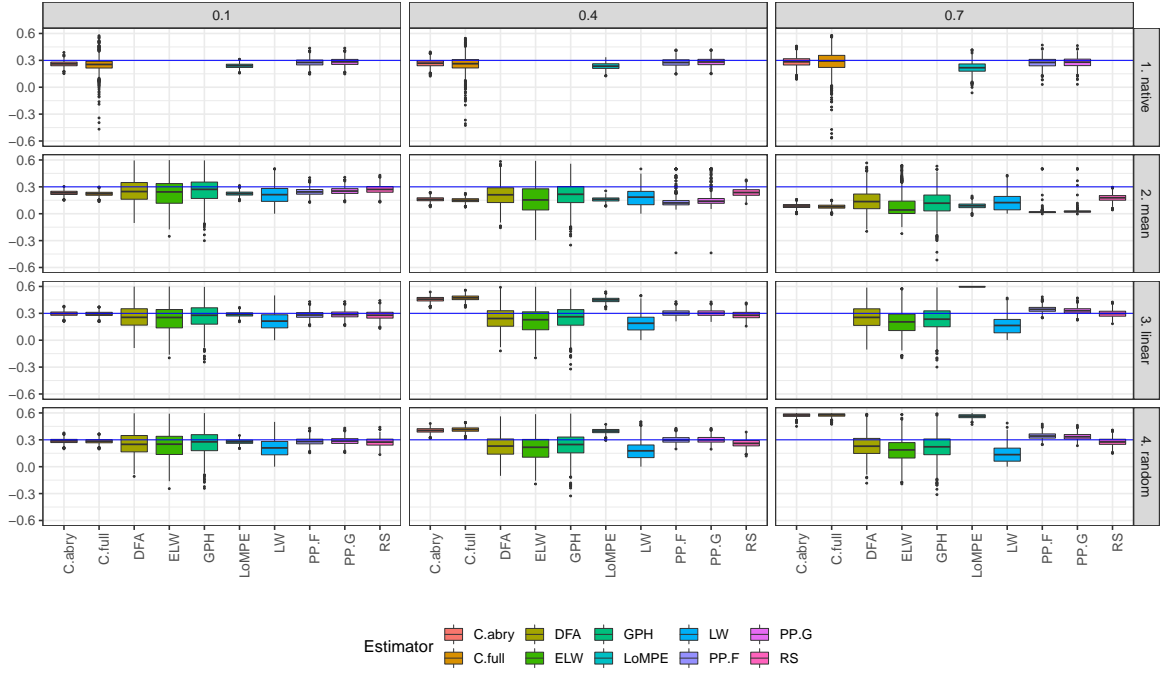

Figure 5: Box plot of the adjusted model ARFIMA  $(1, d, 1)$  for  $d = 0.3$ .

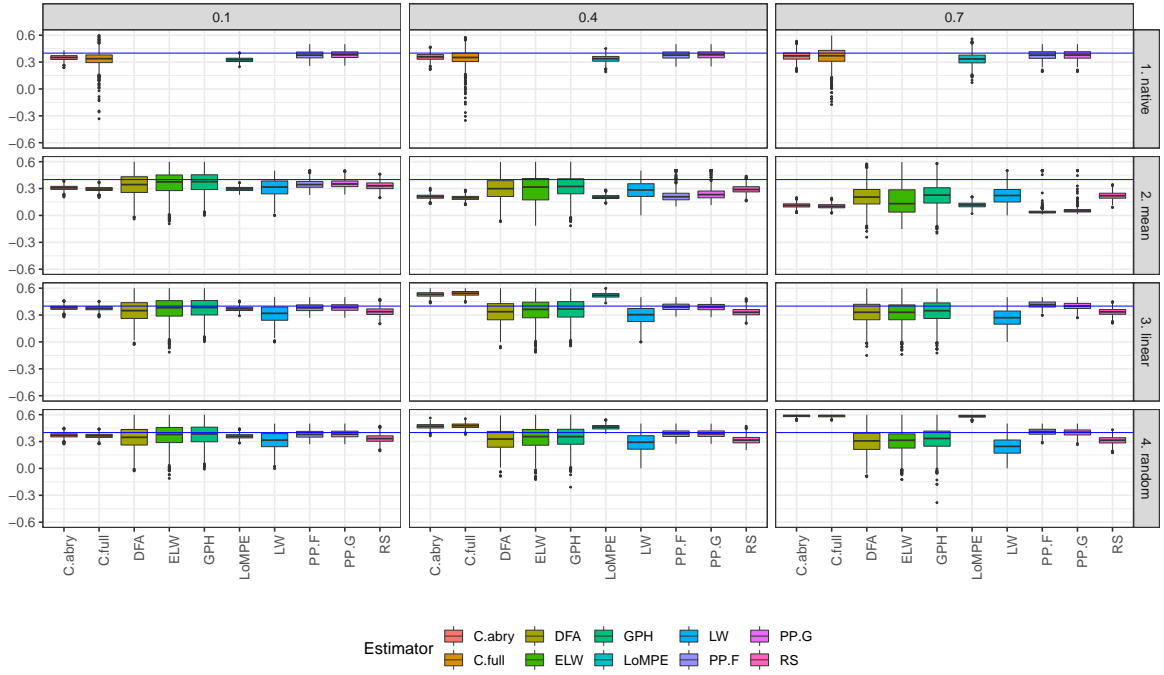

Figure 6: Box plot of the adjusted model ARFIMA  $(1, d, 1)$  for  $d = 0.4$ .

Table 3: Simulation results for the ARFIMA(1, 0.1, 1) scenario.

| $d = 0.1$ |           |              |              |              |              |              |              |              |              |
|-----------|-----------|--------------|--------------|--------------|--------------|--------------|--------------|--------------|--------------|
| Type      | Estimator | Missing      |              |              |              |              |              |              |              |
|           |           | 0            | 0.1          | 0.2          | 0.3          | 0.4          | 0.5          | 0.6          | 0.7          |
| Native    | Full      | 0.076        | 0.077        | 0.086        | 0.088        | 0.109        | 0.113        | <b>0.116</b> | 0.152        |
|           | Abry      | 0.081        | 0.083        | 0.086        | 0.089        | <b>0.096</b> | <b>0.103</b> | <b>0.116</b> | 0.142        |
|           | PP.G      | <b>0.092</b> | <b>0.091</b> | <b>0.091</b> | <b>0.090</b> | 0.088        | 0.086        | <b>0.084</b> | <b>0.073</b> |
|           | PP.F      | 0.086        | 0.086        | 0.086        | 0.085        | 0.083        | 0.081        | 0.080        | 0.071        |
|           | LoMPE     | 0.085        | 0.080        | 0.076        | 0.071        | 0.070        | 0.066        | 0.062        | 0.057        |
| Mean      | Full      | 0.076        | 0.068        | 0.060        | 0.052        | 0.045        | 0.035        | 0.027        | 0.019        |
|           | Abry      | 0.081        | 0.073        | 0.064        | 0.056        | 0.049        | 0.039        | 0.031        | 0.022        |
|           | PP.G      | <b>0.092</b> | 0.075        | 0.057        | 0.043        | 0.062        | 0.054        | 0.012        | 0.007        |
|           | PP.F      | 0.086        | 0.069        | 0.051        | 0.037        | 0.053        | 0.055        | 0.009        | 0.005        |
|           | LoMPE     | 0.085        | <b>0.078</b> | <b>0.070</b> | 0.063        | 0.055        | 0.047        | 0.041        | 0.029        |
|           | DFA       | 0.072        | 0.066        | 0.057        | 0.053        | 0.047        | 0.037        | 0.024        | 0.008        |
|           | GPH       | 0.034        | 0.025        | 0.012        | 0.002        | -0.010       | -0.030       | -0.047       | -0.086       |
|           | LW        | 0.047        | 0.045        | 0.041        | 0.039        | 0.038        | 0.032        | 0.030        | 0.020        |
|           | ELW       | 0.044        | 0.041        | 0.037        | 0.036        | 0.039        | 0.044        | 0.050        | 0.065        |
|           | R/S       | 0.143        | 0.138        | 0.134        | <b>0.130</b> | <b>0.125</b> | <b>0.117</b> | <b>0.109</b> | <b>0.098</b> |
| Linear    | Full      | 0.076        | 0.133        | 0.197        | 0.269        | 0.350        | 0.441        | 0.546        | 0.673        |
|           | Abry      | 0.081        | 0.131        | 0.188        | 0.254        | 0.331        | 0.418        | 0.521        | 0.650        |
|           | PP.G      | <b>0.092</b> | 0.120        | 0.143        | 0.164        | 0.182        | 0.200        | 0.221        | 0.247        |
|           | PP.F      | 0.086        | <b>0.115</b> | 0.139        | 0.161        | 0.183        | 0.205        | 0.233        | 0.266        |
|           | LoMPE     | 0.085        | 0.135        | 0.192        | 0.256        | 0.329        | 0.412        | 0.512        | 0.632        |
|           | DFA       | 0.072        | 0.072        | <b>0.072</b> | <b>0.078</b> | <b>0.083</b> | <b>0.094</b> | <b>0.108</b> | <b>0.134</b> |
|           | GPH       | 0.034        | 0.032        | 0.029        | 0.026        | 0.029        | 0.028        | 0.031        | 0.036        |
|           | LW        | 0.047        | 0.046        | 0.040        | 0.038        | 0.039        | 0.033        | 0.032        | 0.031        |
|           | ELW       | 0.044        | 0.041        | 0.037        | 0.036        | 0.039        | 0.033        | 0.034        | 0.036        |
|           | R/S       | 0.143        | 0.149        | 0.157        | 0.167        | 0.178        | 0.192        | 0.209        | 0.234        |
| Random    | Full      | 0.076        | 0.128        | 0.184        | 0.244        | 0.311        | 0.380        | 0.454        | 0.538        |
|           | Abry      | 0.081        | 0.126        | 0.177        | 0.233        | 0.296        | 0.365        | 0.442        | 0.531        |
|           | PP.G      | <b>0.092</b> | 0.118        | 0.141        | 0.163        | 0.184        | 0.206        | 0.231        | 0.261        |
|           | PP.F      | 0.086        | <b>0.112</b> | 0.136        | 0.160        | 0.183        | 0.208        | 0.236        | 0.271        |
|           | LoMPE     | 0.085        | 0.131        | 0.180        | 0.235        | 0.293        | 0.359        | 0.431        | 0.512        |
|           | DFA       | 0.072        | 0.068        | <b>0.067</b> | <b>0.070</b> | <b>0.072</b> | <b>0.083</b> | <b>0.101</b> | <b>0.130</b> |
|           | GPH       | 0.034        | 0.030        | 0.023        | 0.021        | 0.025        | 0.021        | 0.029        | 0.041        |
|           | LW        | 0.047        | 0.044        | 0.038        | 0.035        | 0.033        | 0.029        | 0.028        | 0.031        |
|           | ELW       | 0.044        | 0.040        | 0.036        | 0.035        | 0.035        | 0.029        | 0.031        | 0.037        |
|           | R/S       | 0.143        | 0.145        | 0.150        | 0.156        | 0.164        | 0.177        | 0.193        | 0.222        |

Table 4: Simulation results for the ARFIMA(1, 0.2, 1) scenario.

| $d = 0.2$ |           |              |              |              |              |              |              |              |              |
|-----------|-----------|--------------|--------------|--------------|--------------|--------------|--------------|--------------|--------------|
| Type      | Estimator | Missing      |              |              |              |              |              |              |              |
|           |           | 0            | 0.1          | 0.2          | 0.3          | 0.4          | 0.5          | 0.6          | 0.7          |
| Native    | Full      | 0.160        | 0.164        | 0.164        | 0.170        | 0.181        | <b>0.190</b> | <b>0.197</b> | 0.225        |
|           | Abry      | 0.167        | 0.171        | 0.171        | 0.175        | 0.178        | 0.182        | 0.185        | <b>0.203</b> |
|           | PP.G      | <b>0.188</b> | <b>0.187</b> | <b>0.186</b> | <b>0.185</b> | <b>0.185</b> | 0.182        | 0.179        | 0.177        |
|           | PP.F      | 0.180        | 0.180        | 0.180        | 0.179        | 0.178        | 0.176        | 0.174        | 0.172        |
|           | LoMPE     | 0.164        | 0.156        | 0.151        | 0.142        | 0.146        | 0.138        | 0.130        | 0.125        |
| Mean      | Full      | 0.160        | 0.146        | 0.130        | 0.114        | 0.098        | 0.083        | 0.064        | 0.048        |
|           | Abry      | 0.167        | 0.152        | 0.136        | 0.121        | 0.105        | 0.089        | 0.070        | 0.053        |
|           | PP.G      | <b>0.188</b> | 0.161        | 0.131        | 0.105        | 0.108        | 0.068        | 0.027        | 0.018        |
|           | PP.F      | 0.180        | 0.152        | 0.120        | 0.092        | 0.091        | 0.072        | 0.021        | 0.013        |
|           | LoMPE     | 0.164        | 0.149        | 0.136        | 0.121        | 0.106        | 0.091        | 0.075        | 0.057        |
|           | DFA       | 0.172        | 0.164        | 0.152        | 0.138        | 0.125        | 0.109        | 0.089        | 0.069        |
|           | GPH       | 0.154        | 0.141        | 0.126        | 0.106        | 0.087        | 0.068        | 0.043        | 0.003        |
|           | LW        | 0.124        | 0.118        | 0.110        | 0.102        | 0.094        | 0.082        | 0.072        | 0.057        |
|           | ELW       | 0.135        | 0.126        | 0.112        | 0.097        | 0.088        | 0.079        | 0.076        | 0.086        |
|           | R/S       | 0.214        | <b>0.207</b> | <b>0.198</b> | <b>0.189</b> | <b>0.178</b> | <b>0.167</b> | <b>0.152</b> | <b>0.135</b> |
| Linear    | Full      | 0.160        | 0.212        | 0.268        | 0.333        | 0.407        | 0.494        | 0.587        | 0.707        |
|           | Abry      | 0.167        | 0.212        | 0.262        | 0.321        | 0.389        | 0.471        | 0.563        | 0.685        |
|           | PP.G      | <b>0.188</b> | <b>0.199</b> | 0.210        | 0.220        | 0.231        | 0.243        | 0.257        | 0.277        |
|           | PP.F      | 0.180        | 0.193        | <b>0.206</b> | <b>0.218</b> | 0.232        | 0.248        | 0.268        | 0.295        |
|           | LoMPE     | 0.164        | 0.208        | 0.259        | 0.317        | 0.385        | 0.463        | 0.554        | 0.666        |
|           | DFA       | 0.172        | 0.170        | 0.164        | 0.159        | 0.160        | 0.161        | <b>0.165</b> | <b>0.189</b> |
|           | GPH       | 0.154        | 0.148        | 0.142        | 0.133        | 0.127        | 0.120        | 0.115        | 0.117        |
|           | LW        | 0.124        | 0.119        | 0.110        | 0.103        | 0.096        | 0.087        | 0.080        | 0.076        |
|           | ELW       | 0.135        | 0.131        | 0.124        | 0.118        | 0.113        | 0.102        | 0.098        | 0.101        |
|           | R/S       | 0.214        | 0.216        | 0.218        | 0.220        | <b>0.225</b> | <b>0.232</b> | 0.242        | 0.261        |
| Random    | Full      | 0.160        | 0.204        | 0.250        | 0.302        | 0.358        | 0.420        | 0.485        | 0.563        |
|           | Abry      | 0.167        | 0.205        | 0.245        | 0.293        | 0.346        | 0.407        | 0.474        | 0.557        |
|           | PP.G      | <b>0.188</b> | <b>0.198</b> | 0.209        | 0.219        | 0.232        | 0.246        | 0.264        | 0.287        |
|           | PP.F      | 0.180        | 0.191        | <b>0.204</b> | 0.216        | 0.231        | 0.248        | 0.269        | 0.297        |
|           | Knight    | 0.164        | <b>0.202</b> | 0.243        | 0.290        | 0.341        | 0.399        | 0.463        | 0.535        |
|           | DFA       | 0.172        | 0.166        | 0.157        | 0.149        | 0.145        | 0.145        | 0.150        | <b>0.172</b> |
|           | GPH       | 0.154        | 0.146        | 0.137        | 0.130        | 0.115        | 0.114        | 0.103        | 0.110        |
|           | LW        | 0.124        | 0.116        | 0.105        | 0.097        | 0.086        | 0.076        | 0.069        | 0.066        |
|           | ELW       | 0.135        | 0.129        | 0.121        | 0.113        | 0.105        | 0.095        | 0.089        | 0.092        |
|           | R/S       | 0.214        | 0.211        | 0.208        | <b>0.207</b> | <b>0.208</b> | <b>0.212</b> | <b>0.225</b> | 0.244        |

Table 5: Simulation results for the ARFIMA(1, 0.3, 1) scenario.

| $d = 0.3$ |           |              |              |              |              |              |              |              |              |
|-----------|-----------|--------------|--------------|--------------|--------------|--------------|--------------|--------------|--------------|
| Type      | Estimator | Missing      |              |              |              |              |              |              |              |
|           |           | 0            | 0.1          | 0.2          | 0.3          | 0.4          | 0.5          | 0.6          | 0.7          |
| Native    | Full      | 0.247        | 0.255        | 0.264        | 0.277        | 0.241        | 0.272        | 0.269        | <b>0.296</b> |
|           | Abry      | 0.256        | 0.261        | 0.263        | 0.264        | 0.266        | 0.270        | 0.273        | 0.283        |
|           | PP.G      | <b>0.283</b> | <b>0.282</b> | <b>0.282</b> | <b>0.281</b> | <b>0.282</b> | <b>0.280</b> | <b>0.277</b> | 0.276        |
|           | PP.F      | 0.277        | 0.277        | 0.276        | 0.276        | 0.276        | 0.275        | 0.273        | 0.273        |
|           | LoMPE     | 0.247        | 0.239        | 0.234        | 0.225        | 0.235        | 0.224        | 0.210        | 0.218        |
| Mean      | Full      | 0.247        | 0.223        | 0.200        | 0.175        | 0.151        | 0.128        | 0.103        | 0.079        |
|           | Abry      | 0.256        | 0.233        | 0.210        | 0.185        | 0.161        | 0.138        | 0.112        | 0.086        |
|           | PP.G      | <b>0.283</b> | 0.253        | 0.217        | 0.180        | 0.171        | 0.094        | 0.058        | 0.029        |
|           | PP.F      | 0.277        | 0.244        | 0.205        | 0.164        | 0.149        | 0.082        | 0.046        | 0.021        |
|           | LoMPE     | 0.247        | 0.225        | 0.202        | 0.181        | 0.159        | 0.136        | 0.113        | 0.088        |
|           | DFA       | 0.268        | 0.257        | 0.243        | 0.229        | 0.212        | 0.196        | 0.167        | 0.138        |
|           | GPH       | 0.273        | 0.259        | 0.246        | 0.225        | 0.208        | 0.176        | 0.150        | 0.112        |
|           | LW        | 0.215        | 0.208        | 0.199        | 0.189        | 0.178        | 0.164        | 0.146        | 0.126        |
|           | ELW       | 0.250        | 0.235        | 0.218        | 0.192        | 0.177        | 0.150        | 0.135        | 0.120        |
|           | R/S       | 0.280        | <b>0.271</b> | <b>0.261</b> | <b>0.249</b> | <b>0.237</b> | <b>0.221</b> | <b>0.201</b> | <b>0.177</b> |
| Linear    | Full      | 0.247        | 0.293        | 0.346        | 0.406        | 0.473        | 0.551        | 0.643        | 0.755        |
|           | Abry      | 0.256        | <b>0.296</b> | 0.342        | 0.395        | 0.457        | 0.531        | 0.621        | 0.733        |
|           | PP.G      | <b>0.283</b> | 0.287        | <b>0.292</b> | <b>0.295</b> | <b>0.301</b> | <b>0.307</b> | 0.315        | 0.328        |
|           | PP.F      | 0.277        | 0.282        | 0.288        | 0.293        | 0.303        | 0.312        | 0.325        | 0.345        |
|           | LoMPE     | 0.247        | 0.288        | 0.333        | 0.386        | 0.448        | 0.520        | 0.603        | 0.711        |
|           | DFA       | 0.268        | 0.262        | 0.258        | 0.252        | 0.247        | 0.247        | 0.247        | 0.258        |
|           | GPH       | 0.273        | 0.269        | 0.265        | 0.252        | 0.250        | 0.235        | 0.227        | 0.233        |
|           | LW        | 0.215        | 0.210        | 0.204        | 0.193        | 0.186        | 0.173        | 0.165        | 0.160        |
|           | ELW       | 0.250        | 0.245        | 0.240        | 0.227        | 0.222        | 0.208        | 0.204        | 0.201        |
|           | R/S       | 0.280        | 0.279        | 0.279        | 0.278        | 0.280        | 0.282        | <b>0.286</b> | <b>0.297</b> |
| Random    | Full      | 0.247        | 0.284        | 0.324        | 0.367        | 0.415        | 0.468        | 0.527        | 0.593        |
|           | Abry      | 0.256        | <b>0.287</b> | 0.322        | 0.360        | 0.405        | 0.458        | 0.518        | 0.589        |
|           | PP.G      | <b>0.283</b> | 0.286        | <b>0.291</b> | <b>0.294</b> | 0.301        | <b>0.308</b> | <b>0.318</b> | 0.334        |
|           | PP.F      | 0.277        | 0.281        | 0.286        | 0.291        | <b>0.300</b> | 0.309        | 0.323        | 0.343        |
|           | LoMPE     | 0.247        | 0.279        | 0.313        | 0.352        | 0.398        | 0.446        | 0.500        | 0.567        |
|           | DFA       | 0.268        | 0.259        | 0.252        | 0.238        | 0.231        | 0.227        | 0.227        | 0.233        |
|           | GPH       | 0.273        | 0.266        | 0.263        | 0.245        | 0.239        | 0.221        | 0.215        | 0.216        |
|           | LW        | 0.215        | 0.207        | 0.200        | 0.186        | 0.175        | 0.158        | 0.149        | 0.139        |
|           | ELW       | 0.250        | 0.242        | 0.237        | 0.219        | 0.210        | 0.195        | 0.191        | 0.182        |
|           | R/S       | 0.280        | 0.274        | 0.269        | 0.263        | 0.261        | 0.261        | 0.264        | <b>0.277</b> |

Table 6: Simulation results for the ARFIMA(1, 0.4, 1) scenario.

| $d = 0.4$ |           |              |              |              |              |              |              |              |              |
|-----------|-----------|--------------|--------------|--------------|--------------|--------------|--------------|--------------|--------------|
| Type      | Estimator | Missing      |              |              |              |              |              |              |              |
|           |           | 0            | 0.1          | 0.2          | 0.3          | 0.4          | 0.5          | 0.6          | 0.7          |
| Native    | Full      | 0.332        | 0.341        | 0.347        | 0.346        | 0.353        | 0.358        | 0.366        | 0.365        |
|           | Abry      | 0.344        | 0.350        | 0.352        | 0.355        | 0.358        | 0.360        | 0.362        | 0.366        |
|           | PP.G      | <b>0.384</b> | <b>0.383</b> | <b>0.383</b> | <b>0.383</b> | <b>0.382</b> | <b>0.380</b> | <b>0.380</b> | <b>0.378</b> |
|           | PP.F      | 0.381        | 0.380        | 0.380        | 0.381        | 0.380        | 0.378        | 0.379        | <b>0.378</b> |
|           | LoMPE     | 0.332        | 0.325        | 0.322        | 0.314        | 0.336        | 0.325        | 0.312        | 0.334        |
| Mean      | Full      | 0.332        | 0.294        | 0.260        | 0.227        | 0.196        | 0.165        | 0.133        | 0.102        |
|           | Abry      | 0.344        | 0.307        | 0.274        | 0.241        | 0.209        | 0.178        | 0.144        | 0.112        |
|           | PP.G      | 0.384        | 0.354        | 0.317        | 0.277        | 0.253        | 0.102        | 0.114        | 0.062        |
|           | PP.F      | 0.381        | 0.348        | 0.307        | 0.261        | 0.229        | 0.086        | 0.092        | 0.046        |
|           | LoMPE     | 0.332        | 0.297        | 0.265        | 0.234        | 0.205        | 0.175        | 0.145        | 0.117        |
|           | DFA       | 0.367        | 0.355        | 0.344        | 0.326        | 0.305        | 0.274        | 0.251        | 0.213        |
|           | GPH       | <b>0.393</b> | <b>0.379</b> | <b>0.363</b> | <b>0.346</b> | <b>0.323</b> | <b>0.292</b> | <b>0.267</b> | <b>0.220</b> |
|           | LW        | 0.317        | 0.311        | 0.303        | 0.295        | 0.280        | 0.263        | 0.246        | 0.218        |
|           | ELW       | 0.380        | 0.368        | 0.353        | 0.332        | 0.303        | 0.276        | 0.234        | 0.204        |
|           | R/S       | 0.341        | 0.332        | 0.321        | 0.308        | 0.291        | 0.271        | 0.249        | <b>0.220</b> |
| Linear    | Full      | 0.332        | 0.375        | 0.424        | 0.481        | 0.544        | 0.617        | 0.702        | 0.807        |
|           | Abry      | 0.344        | 0.381        | 0.423        | 0.473        | 0.531        | 0.599        | 0.681        | 0.786        |
|           | PP.G      | 0.384        | 0.385        | <b>0.386</b> | 0.388        | 0.389        | 0.391        | <b>0.396</b> | <b>0.402</b> |
|           | PP.F      | 0.381        | 0.383        | <b>0.386</b> | <b>0.389</b> | <b>0.392</b> | <b>0.397</b> | 0.406        | 0.417        |
|           | LoMPE     | 0.332        | 0.371        | <b>0.414</b> | 0.462        | 0.520        | 0.587        | 0.664        | 0.765        |
|           | DFA       | 0.367        | 0.364        | 0.362        | 0.355        | 0.350        | 0.342        | 0.345        | 0.347        |
|           | GPH       | <b>0.393</b> | <b>0.391</b> | 0.385        | 0.382        | 0.375        | 0.363        | 0.359        | 0.353        |
|           | LW        | 0.317        | 0.314        | 0.311        | 0.305        | 0.298        | 0.286        | 0.278        | 0.269        |
|           | ELW       | 0.380        | 0.376        | 0.372        | 0.364        | 0.356        | 0.345        | 0.336        | 0.329        |
|           | R/S       | 0.341        | 0.339        | 0.336        | 0.335        | 0.332        | 0.330        | 0.332        | 0.335        |
| Random    | Full      | 0.332        | 0.363        | 0.397        | 0.436        | 0.476        | 0.522        | 0.571        | 0.628        |
|           | Abry      | 0.344        | 0.369        | <b>0.398</b> | 0.432        | 0.470        | 0.513        | 0.565        | 0.626        |
|           | PP.G      | 0.384        | 0.384        | 0.386        | <b>0.387</b> | 0.388        | 0.390        | 0.397        | <b>0.404</b> |
|           | PP.F      | 0.381        | 0.382        | 0.384        | 0.386        | <b>0.389</b> | <b>0.393</b> | <b>0.401</b> | 0.412        |
|           | LoMPE     | 0.332        | 0.359        | 0.389        | 0.422        | 0.460        | 0.502        | 0.547        | 0.605        |
|           | DFA       | 0.367        | 0.361        | 0.355        | 0.344        | 0.334        | 0.323        | 0.321        | 0.315        |
|           | GPH       | <b>0.393</b> | <b>0.388</b> | 0.382        | 0.374        | 0.363        | 0.354        | 0.343        | 0.331        |
|           | LW        | 0.317        | 0.312        | 0.307        | 0.298        | 0.287        | 0.273        | 0.260        | 0.244        |
|           | ELW       | 0.380        | 0.373        | 0.369        | 0.358        | 0.345        | 0.329        | 0.318        | 0.305        |
|           | R/S       | 0.341        | 0.334        | 0.328        | 0.321        | 0.316        | 0.310        | 0.311        | 0.314        |
